# Supplementary material for: Unsupervised dynamic modeling of medical image transformation
Source: arXiv:2103.00930 source file (2022-11-07)
Supplement: Supplementary file 1 [file Appendix.tex]

\appendix
\section{Evidence lower bound derivation}
\subsection{Variational Auto-Encoder}
\label{appendix_vae}
%The log likelihood for VAE is in general intractable 

%\begin{equation}
%\begin{split}
%    p_\theta(y) & = \int_x p_\theta(x, y) \\
%    & = \int_x p_\theta(y \mid x) p_\theta(x) \\
%    & = \int_x \dfrac{p_\theta(y)p_\theta(x \mid y)}{p_\theta(x)} p_\theta(x)
%\end{split}
%\end{equation}
With approximate inference techniques approximations of the posterior is possible. From the KL divergence between the variational approximation posterior, $q_\phi(x \mid y)$ and the true posterior $p_\theta(x \mid y)$ we get

\begin{equation}
    \begin{split}
        0 & \leq \KL \Big( q_\phi(x \mid y) || p_\theta(x \mid y) \Big) = \E_{q_\phi(x \mid y)} \Big[ \log \dfrac{q_\phi(x\mid y)}{p_\theta(x \mid y)} \Big] \\
        & = \E_{q_\phi(x \mid y)} \Big[ \log \dfrac{q_\phi(x\mid y)p(y)}{p_\theta(x, y)} \Big] = \E_{q_\phi(x \mid y)} \Big[ \log \dfrac{q_\phi(x\mid y)}{p_\theta(x, y)} \Big] + \log p(y).
    \end{split}
    \label{eq:dkl_vae}
\end{equation}
Moving the expectation to the other side and we obtain the evidence lower bound (ELBO) of the marginal log likelihood, $\log p_\theta(y)$:
\begin{equation}
    \begin{split}
        \log p_\theta(y) & \geq -\E_{q_\phi(x \mid y)} \Big[\log \dfrac{q_\phi(x\mid y)}{p_\theta(x, y)}\Big] \\
        & = \E_{q_\phi(x \mid y)} \Big[\log \dfrac{p_\theta(x, y)}{q_\phi(x\mid y)}\Big] \\
        & = \E_{q_\phi(x \mid y)} \Big[ \log p_\theta(x, y) - \log q_\phi(x\mid y) \Big].
    \end{split}
    \label{eq:loss_vae}
\end{equation}
\subsection{Kalman Variational Auto-Encoder}
\label{appendix_kvae}
Similar as for the traditional VAE the KL divergence between the approximate and real posterior distribution is given by
\begin{equation}
    \begin{split}
        0 & \leq \KL\Big(q_{\phi, \gamma}(\vx,\vz \mid \vy) || p_{\theta, \gamma}(\vx, \vz \mid \vy)\Big) \\
        & = 
        \E_{q_{\phi,\gamma}(\vx, \vz\mid \vy)}\Big[ \log \dfrac{q_{\phi, \gamma}(\vx, \vz \mid \vy)}{p_{\theta, \gamma}(\vx, \vz \mid \vy)}\Big] \\
        & = 
        \E_{q_{\phi,\gamma}(\vx, \vz\mid \vy)}\Big[ \log \dfrac{q_{\phi, \gamma}(\vx, \vz \mid \vy)p_{\theta, \gamma}(\vy)}{p_{\theta, \gamma}(\vx, \vz, \vy)}\Big] \\
        & = \E_{q_{\phi,\gamma}(\vx, \vz\mid \vy)}\Big[ \log \dfrac{q_{\phi, \gamma}(\vx, \vz \mid \vy)}{p_{\theta, \gamma}(\vx, \vz, \vy)}\Big] + \log p_{\theta, \gamma}(\vy).
    \end{split}
\end{equation}
Moving the expectation to the other side and we obtain the evidence lower bound (ELBO) of the marginal log likelihood, $\log p_{\theta, \gamma}(\vy)$:
\begin{equation}
\begin{split}
    \log p_{\theta, \gamma}(\vy) & \geq 
    -\E_{q_{\phi,\gamma}(\vx, \vz\mid \vy)}\Big[ \log \dfrac{q_{\phi, \gamma}(\vx, \vz \mid \vy)}{p_{\theta, \gamma}(\vx, \vz, \vy)}\Big] \\
    & = \E_{q_{\phi,\gamma}(\vx, \vz\mid \vy)}\Big[ \log \dfrac{p_{\theta, \gamma}(\vx, \vz, \vy)}{q_{\phi, \gamma}(\vx, \vz \mid \vy)}\Big] \\
    & = \E_{q_{\phi,\gamma}(\vx, \vz\mid \vy)}\Big[ \log p_{\theta, \gamma}(\vx, \vz, \vy) - \log q_{\phi, \gamma}(\vx, \vz \mid \vy)\Big], \\
\end{split}
\label{eq_ap_kvae_elbo}
\end{equation}
where the joint distribution
\begin{equation}
    \begin{split}
        p_{\theta, \gamma}(\vx, \vz, \vy) = p_\theta(\vy \mid \vx) p_\gamma(\vx, \vz),
    \end{split}
\end{equation}
and 
\begin{align*}
        & p_\theta(\vy \mid \vx) = \prod_{t=1}^T p_\theta(y_t \mid x_t) , \quad
        & p_\gamma(\vx, \vz) = \prod_{t=1}^T p_\gamma(x_t \mid z_t) \cdot p_\gamma(z_1) \prod_{t=2}^T p_\gamma(z_t \mid z_{t  -1}).
\end{align*}
For Kalman Variational Autoencoders the posterior is approximated as
\begin{equation}
    \begin{split}
        q_{\phi, \gamma}(\vx, \vz \mid \vy) & = p_\gamma(\vz \mid \vx) q_\phi (\vx \mid \vy) = \prod_{t=1}^T p_\gamma(z_t \mid \vx) \prod_{t=1}^T q_\phi (x_t \mid y_t),
    \end{split}
\end{equation}
%NEW?
%\begin{equation}
%    \begin{split}
%        q_{\phi, \gamma}(\vx, \vz \mid \vy) & = p_\gamma(\vz \mid \vx) q_\phi (\vz \mid \vy, \vx) = \prod_{t=1}^T p_\gamma(z_t \mid \vx) \prod_{t=1}^T q_\phi (x_t \mid y_t)
%    \end{split}
%\end{equation}
where $p_\gamma(z_t \mid \vx)$ is given in closed form by the Kalman smoother algorithm (see \ref{appendix_kalman}) and $q_\phi (x_t \mid y_t)$ is given by the encoder. We can now rewrite (\ref{eq_ap_kvae_elbo}) as
\begin{equation}
    \begin{split}
        \log p_{\theta, \gamma}(\vy) & \geq \E_{q_{\phi,\gamma}(\vx, \vz\mid \vy)}\Big[ \log p_{\theta, \gamma}(\vx, \vz, \vy) - \log q_{\phi, \gamma}(\vx, \vz \mid \vy)\Big] \\
        & = \E_{q_{\phi,\gamma}(\vx, \vz\mid \vy)}\Big[ \log p_\theta(\vy\mid \vx) p_\gamma(\vx, \vz) - \log p_\gamma(\vz \mid \vx) q_\theta(\vx \mid \vy)\Big] \\
        & = \E_{q_{\phi,\gamma}(\vx, \vz\mid \vy)}\Big[
        \log \dfrac{p_\theta(\vy\mid \vx)}{q_\theta(\vx\mid \vy)} + \dfrac{p_\gamma(\vx,\vz)}{p_\gamma(\vz \mid \vx)}\Big] \\
        & = \E_{q_{\phi}(\vx\mid \vy)}\Big[
        \log \dfrac{p_\theta(\vy\mid \vx)}{q_\theta(\vx\mid \vy)} + 
        \E_{p_\gamma(\vz\mid \vx)}\Big[ \dfrac{p_\gamma(\vx, \vz)}{p_\gamma(\vz \mid \vx)}\Big]\Big].
    \end{split}
\end{equation}

\section{Kalman filter and smoother}
\label{appendix_kalman}
The Kalman filter and smoothing algorithm is given by

\begin{algorithm2e}[H]
\caption{Kalman filtering}
\label{alg:kalman_filter}
\DontPrintSemicolon 
\KwIn{$x_1, \ldots, x_T, \mu_{1\mid0}, \Sigma_{1\mid 0}, A,C,Q,R$}
\KwOut{$\mu_{t+1 \mid t}, \Sigma_{t+1 \mid t}, \mu_{t \mid t}, \Sigma_{t \mid t}$ for $t = [1, \dots, T]$}
$y\gets 0$\;
\For{$t\gets 1$ \KwTo $T$}{
  Measurement Update \;
  $K_t \gets \Sigma_{t \mid t-1} C^T(C \Sigma_{t \mid t-1}C^T + R)^{-1}$ \;
  $\mu_{t\mid t} \gets \mu_{t\mid t-1} + K_t(x_t - C \mu_{t \mid t-1})$ \;
  $\Sigma_{t\mid t} \gets (I - K_t C)\Sigma_{t\mid t-1}(I - K_t C)^T + K_t R K_t^T$ \;
  Time Update \;
  $\mu_{t+1\mid t} \gets A \mu_{t\mid t}$ \;
  $\Sigma_{t+1\mid t} \gets A \Sigma_{t\mid t}A^T + Q$\;
}
\end{algorithm2e}

%\begin{algorithm2e}
%\caption{Square root Kalman filtering}
%\label{alg:kalman_filter_sq}
%\KwIn{$x_1, \ldots, x_T, \mu_{1\mid0}, \Sigma_{1\mid 0}^{1/2}, A,C,Q^{1/2},R^{1/2}$}
%\KwOut{$\mu_{t+1 \mid t}, \Sigma_{t+1 \mid t}^{1/2}, \mu_{t \mid t}, \Sigma_{t \mid t}^{1/2}$ for $t = [1, \dots, T]$}
%$y\leftarrow 0$\;
%\For{$t\leftarrow 1$ \KwTo $T$}{
%Measurement Update\;
%  QR factorisation\;
%  $\begin{bmatrix} \mathcal{R}_{11} & \mathcal{R}_{12} \\ \mathbf{0} & \mathcal{R}_{22} \end{bmatrix} = 
%  \mathcal{Q} \begin{bmatrix}
%  R^{1/2} & \mathbf{0} \\
%  \Sigma_{t\mid t-1}^{1/2}C^T & \Sigma_{t\mid t-1}^{1/2}
%  \end{bmatrix}$ \;
%  $\Sigma_{t+1\mid t} \leftarrow \mathcal{R}_{22}$\;
%  $\mu_{t\mid t} \leftarrow \mu_{t\mid t-1} + \mathcal{R}_{12}^T \mathcal{R}_{11}^{-T}(x_t - C \mu_{t \mid t-1})$ \;
%  Time Update\;
%  QR factorisation\;
%  $\begin{bmatrix}\bar{\mathcal{R}} \\ \mathbf{0}\end{bmatrix} = 
%  \bar{\mathcal{Q}} \begin{bmatrix}
%  \Sigma_{t\mid t}^{1/2} A^T \\ Q^{1/2} \end{bmatrix}$\;
%  $\Sigma_{t+1\mid t}^{1/2} \leftarrow \bar{\mathcal{R}}$\;
%  $\mu_{t+1\mid t} \leftarrow A\mu_{t\mid t}$
%}
%\end{algorithm2e}

\begin{algorithm2e}[H]
\caption{Kalman smoothing}
\label{alg:kalman_smooth}
\DontPrintSemicolon 
\KwIn{$\mu_{t+1\mid t}, \Sigma_{t+1\mid t}, \mu_{t\mid t}, \Sigma_{t\mid t}$ for $t = [1, \dots, T], A$}
\KwOut{$\mu_{t \mid T}, \Sigma_{t \mid T}$ for $t = [0, \dots, T-1]$}
\For{$t\gets T-1$ \KwTo $0$}{
  $L_t \gets \Sigma_{t \mid t}A^T\Sigma_{t+1 \mid t}^{-1}$ \;
  $\mu_{t\mid T} \gets \mu_{t \mid t} + L_t(\mu_{t+1\mid T} -  \mu_{t+1\mid t})$ \;
  $\Sigma_{t \mid T} \gets \Sigma_{t \mid t} + L_t(\Sigma_{t+1\mid T} - \Sigma_{t+1\mid t})L_t^T$ \;
}
\end{algorithm2e}
